# Supplementary material for: AGLLDiff: Guiding Diffusion Models Towards Unsupervised Training-free Real-world Low-light Image Enhancement
Source: arXiv:2407.14900 source file (2024-07-23)
Supplement: Supplementary file 1 [file X_suppl.tex]

\clearpage
\setcounter{page}{1}
\maketitlesupplementary

\section{More Technical Details}
\begin{figure}[!t]
    \centering
\setlength{\abovecaptionskip}{0.1cm} %调整caption与图的距离
    \setlength{\belowcaptionskip}{-0.2cm}%调整caption与下文的距离
    \includegraphics[width=1\linewidth]{figs/subliment1.png}
    \caption{Procedure of the lookup and trilinear interpolation. Each  element $P_{\left( i,j,k \right)}$ denotes an indexing RGB color $\left\{ I_{(i,j,k)}^{r},I_{(i,j,k)}^{g},I_{(i,j,k)}^{b} \right\}$ and the corresponding transformed output RGB color $\left\{ O_{(i,j,k)}^{r},O_{(i,j,k)}^{g},O_{(i,j,k)}^{b} \right\}$.}
    \label{lookup}
\end{figure}
\subsection{Lookup and Trilinear Interpolation} 
% \textbf{Noise-aware trilinear interpolation.} 
In this study, the 3D-LUT can be represented as a discrete sampling of a complete 3D color transform function, encompassing a total of $N^3$ sampling points in space. The sampled results are stored in a 3D lattice of output color values $\left\{ O_{(i,j,k)}^{r},O_{(i,j,k)}^{g},O_{(i,j,k)}^{b} \right\} 
$ that can be queried by sets of input color coordinates $\left\{ I_{(i,j,k)}^{r},I_{(i,j,k)}^{g},I_{(i,j,k)}^{b} \right\}$. Once sampling elements in the 3D-LUT, the input color look up its nearest eight sampling points based on its index and calculate its transformed output by trilinear interpolation~\cite{3DLUT}.

Specifically, to identify the eight nearest adjacent elements surrounding a specific input index in a 3D-LUT, we first calculate this index $(i, j, k)$ using the input RGB values $\left\{ I_{(x,y,z)}^{r},I_{(x,y,z)}^{g},I_{(x,y,z)}^{b} \right\}$. This computation process unfolds as follows:
\begin{equation}
\begin{array}{c}
	x=\frac{I_{(x,y,z)}^{r}}{\Delta},y=\frac{I_{(x,y,z)}^{g}}{\Delta},z=\frac{I_{(x,y,z)}^{b}}{\Delta}\\
	i=\lfloor x \rfloor ,j=\lfloor y \rfloor ,k=\lfloor z \rfloor\\
\end{array},
\label{index}
\end{equation}
where $\Delta =V_{max}/N$, $V_{max}$ denotes the maximum color value. $\lfloor \cdot \rfloor$ signifies the floor function. Then, the offset between the input precise index $(x, y, z)$ and the computed sampling point $(i, j, k)$ can be computed:
\begin{equation}
    d_x=x-i, d_y=y-j, d_z=z-k.
\label{distance}
\end{equation}

Combining the Equation \ref{index} and Equation \ref{distance}, we derive the interpolated output as follows. Figure \ref{lookup} graphically demonstrates this interpolation process:
\begin{equation}
\begin{aligned}
	O_{(i,j,k)}^{c}&=\left( 1-d_x \right) \left( 1-d_y \right) \left( 1-d_z \right) O_{(i,j,k)}^{c}\\
	&+d_x\left( 1-d_y \right) \left( 1-d_z \right) O_{(i+1,j,k)}^{c}\\
	&+\left( 1-d_x \right) d_y\left( 1-d_z \right) O_{(i,j+1,k)}^{c}\\
	&+\left( 1-d_x \right) \left( 1-d_y \right) d_zO_{(i,j,k+1)}^{c}\\
	&+d_xd_y\left( 1-d_z \right) O_{(i+1,j+1,k)}^{c}\\
	&+\left( 1-d_x \right) d_yd_zO_{(i,j+1,k+1)}^{c}\\
	&+d_x\left( 1-d_y \right) d_zO_{(i+1,j,k+1)}^{c}\\
	&+d_xd_yd_zO_{(i+1,j+1,k+1)}^{c}\\
\end{aligned},
\end{equation}
where $c$ is an element of the set $\{r,g,b\}$. Notably, this interpolation operation is differentiable, allowing for the update of LUTs during end-to-end training.

\begin{figure}[!t]
    \centering
\setlength{\abovecaptionskip}{0.1cm} %调整caption与图的距离
    \includegraphics[width=1\linewidth]{figs/ablation3.png}
    \caption{Ablation studies on different widths of the predictor network. The red box is the coarse normal-light image, and the gray box is the enhanced version. Notably, $r=0$ signifies that the model operates without the noise-aware map.}
    \label{ablation3}
\end{figure}

\section{Additional Ablation}
In order to fully understand the proposed DPLUT, we present a more exhaustive set of ablation studies on the LOL dataset~\cite{RetinexNet}.
% when the order of the curve mapping function is more high 
% the curve mapping is already very powerful, and continuing to increase the order is not very rewarding, but rather increases the burden of the inference computation.

\subsection{Effectiveness of the Noise-aware Map}
The noise-aware weight map is estimated by a lightweight predictor network. Its architecture is listed in Table \ref{architecture2}. We analyze the impact of the noise-aware weight map by adjusting the network width. As shown in Figure \ref{ablation3}, enlarging the width of the predictor network will improve its capability in noise removal. Meanwhile, the number of parameters also increases. These ablation results confirm the effectiveness of the noise-aware weight map, which can assist the NLUT in suppressing noise. Given the trade-off between memory footprint and denoising performance, the width of the predictor network is configured to 16. Furthermore, we provide the visualization of the noise-aware weight map in Figure \ref{noise_awar_map}.

\begin{table}[!t]
\setlength{\abovecaptionskip}{0.1cm} %调整caption与图的距离
\setlength{\belowcaptionskip}{-0.2cm}%调整caption与下文的距离
\centering
\caption{Architecture of the predictor network, where $r$ is a hyper-parameter that serves as a channel multiplier controlling the width of each convolutional layer. $H \times W$ is the shape of the original image.}\label{architecture2}
% \resizebox{7.5cm}{!}{
% \scalebox{1}{
\setlength\tabcolsep{16.5pt}

\begin{tabular}{ccc}
% \toprule[2pt]
\rowcolor{mygray}
\hline ID  & Layer  & Output Shape  \\
\hline 0 & \text { Bilinear Resize } & $3 \times 256 \times 256$ \\
1 &  Conv3x3, ReLU  & $r \times 128 \times 128$ \\
2 &  Conv3x3, ReLU  & $r \times 256 \times 256 $\\
3 &  Conv3x3, ReLU  & $r \times 256 \times 256 $\\
4 &  Conv3x3, ReLU  & $r \times 256 \times 256 $\\
5 &  Conv3x3, ReLU  & $r \times 256 \times 256 $\\
6 &  Conv3x3, ReLU  & $3 \times 256 \times 256 $\\
7&  \text { Bilinear Resize }  & $3 \times H \times W$ \\
\hline
% \bottomrule[ 2pt]
\end{tabular}
\end{table}

\begin{table}[!t]
\centering
\setlength{\abovecaptionskip}{0.1cm} %调整caption与图的距离
\setlength{\belowcaptionskip}{-0.2cm}%调整caption与下文的距离
\caption{Ablation study on different curve steps. The inference time is evaluated using a single Titan RTX GPU on the image with 4K ($3840 \times 2160$) resolution. The best are marked in \textbf{bold}.}\label{ablation_curve}
% \resizebox{8cm}{!}{
\setlength\tabcolsep{9pt}

\begin{tabular}{c|cccc}
    \hline	\rowcolor{mygray}	
    Steps & PSNR$\uparrow$ & SSIM$\uparrow$ & LPIPS$\downarrow$ &Time (s)$\downarrow$\\
    \hline			
    3 & 9.95 & 0.41 & 0.44&  \textbf{7.7} \\
    5 & 13.11 & 0.58 & 0.31 & 12.5\\
    6 & 13.23 & 0.59 & 0.31 &  15.0\\   
    7 & 18.57 & 0.71 & 0.25 &  17.3\\   
    8 & 20.66 & \textbf{0.74}  & 0.22 &  19.8\\   
    16 & \textbf{20.79} & 0.74 & \textbf{0.21}&  39.2 \\   
    \hline
\end{tabular}
\end{table}

\subsection{Imapct of Curve Steps}
We investigate the effect of varying the number of curve steps on illumination enhancement. As depicted in Figure \ref{ablation4}, increasing the number of curve steps yields progressively improved visual results with natural exposure and refined texture details. Such improvement results are attributed to higher-order curve mapping functions, which possess powerful adjustment capability~\cite{ZeroDCE}. The quantitative results reported in Table \ref{ablation_curve}, indicate that the optimal number of curve steps should not be excessively large. Additionally, a larger number of curve steps correlates with increased computational demands, thereby extending the inference time. Consequently, to balance efficiency with enhancement performance, we set the curve steps to 8.

\section{More Analysis}
\subsection{User Study}
We conducted a user study to more comprehensively evaluate the visual quality of enhanced results obtained by different methods. Specifically, we collected 86 images from the DICM (69 images) \cite{DICM} and MEF (17 images) \cite{MEF} as the evaluation set. For each image, we provided the input low-light image, the corresponding images enhanced by our method, and a baseline. A total of 20 participants were invited to select their preferred image. We select six representative methods for comparison, including 3DLUT~\cite{3DLUT}, ZeroDCE~\cite{ZeroDCE}, ZeroDCE++~\cite{Zerodcepp}, NeRCo~\cite{Neco}, CLIP-LIT~\cite{clip-lie} and PairLIE~\cite{pairLIE}. We report the statistics of the user study in Figure \ref{result3}. The proposed method is preferred by users over all the competing methods, indicating that our method can generate more visually pleasing results.
% To further verify the generalization performance of each method, we conduct experiments on the DICM \cite{DICM} and MEF \cite{MEF} datasets, which contain 69 and 17 low-light images, respectively. Since the above datasets do not include reference images, we perform a user study to understand how users prefer the results of different approaches. 
% Specifically, we conduct the user study based on a pairwise comparison scheme. A total of 20 participants are invited to the test. For each low-light image, two enhanced versions constitute a pair for comparison. Participants are asked to choose the better one from each presented pair. To avoid fatigue and ensure a high-quality subjective evaluation, we select six representative methods for comparison including 3DLUT~\cite{3DLUT}, ZeroDCE~\cite{ZeroDCE}, ZeroDCE++~\cite{Zerodcepp}, NeRco~\cite{Neco}, CLIP-LIE~\cite{clip-lie} and PairLIE~\cite{pairLIE}. 
% We report the average selected times in Figure \ref{result3}.

\begin{figure}[!t]
    \centering
\setlength{\abovecaptionskip}{0.1cm} %调整caption与图的距离
    \includegraphics[width=1\linewidth]{figs/noise_awar_map.png}
    \caption{Visual results of the noise-aware weight map. In each row, the first is the coarse normal-light image, and the other three are visualizations for different channels. Red pixels indicate more activation, and blue pixels indicate less activation.}
    \label{noise_awar_map}
\end{figure}

\begin{figure}[!t]
    \centering
\setlength{\abovecaptionskip}{0.1cm} %调整caption与图的距离
    \includegraphics[width=1\linewidth]{figs/ablation4.png}
    \caption{Ablation studies on different numbers of curve steps ($n$).}
    \label{ablation4}
\end{figure}

\begin{table*}[!t]
\centering
\setlength{\abovecaptionskip}{0.1cm} %调整caption与图的距离
\setlength{\belowcaptionskip}{-0.4cm}%调整caption与下文的距离
\caption{The average perception scores of different approaches on five benchmarks. The best and the second best results are highlighted in \textcolor{red}{red} and \textcolor{blue}{blue} respectively. `-' denotes unavailable.}\label{clip_table}
\resizebox{17.5cm}{!}{
% \scalebox{0.78}{
\setlength\tabcolsep{4pt}

		\begin{tabular}{c|cccccccccccccc}
			\hline \rowcolor{mygray}
			~ & ~ &\multicolumn{1}{c}{SDD} & \multicolumn{1}{c}{LECARM} & \multicolumn{1}{c}{CUE }  & \multicolumn{1}{c}{Retinexformer }& \multicolumn{1}{c}{3DLUT }  &\multicolumn{1}{c}{ZeroDCE} & \multicolumn{1}{c}{ZeroDCE++} &\multicolumn{1}{c}{SCI} & \multicolumn{1}{c}{NeRCo} & \multicolumn{1}{c}{ PairLIE }&  \multicolumn{1}{c}{CLIP-LIT} &~&~ \\ \rowcolor{mygray}	
			 \multirow{-2}*{Datasets}  & \multirow{-2}*{Input}
         &  ~\cite{SDD}  &  ~\cite{LECARM}  &  ~\cite{CUE}  &  ~\cite{Retinexformer}   &~\cite{3DLUT}   &  ~\cite{ZeroDCE}  &  ~\cite{Zerodcepp}  &  ~\cite{SCI} &  ~\cite{Neco}  &  ~\cite{pairLIE} &  ~\cite{clip-lie} & \multirow{-2}*{Ours} & \multirow{-2}*{Reference}\\
			\hline
    LOL~\cite{RetinexNet} & 0.4583 & 0.4718 & 0.4807   & 0.5212 & 0.5374  &0.5168   & 0.5218 & 0.5241 & 0.5184 & 0.5297 & 0.5287 & 0.4987 &\textcolor{blue}{0.5987} & \textcolor{red}{0.6174}\\
    SICE~\cite{SICE}  & 0.4723  & 0.4879 & 0.4921 & 0.5285 & 0.5844  &0.4845  & 0.5283 & 0.5317  &  0.4619 &0.5218 &  0.5316& 0.5011&\textcolor{blue}{0.5504} & \textcolor{red}{0.6370}\\
    LSRW~\cite{LSRW}  & 0.4503  & 0.4692 & 0.4985 & 0.4958 & 0.5233& 0.4766 & 0.4765 & 0.4812 &0.5087& 0.5710 & 0.5296 & 0.4835 &\textcolor{blue}{0.5846} & \textcolor{red}{0.6937}  \\
  DICM~\cite{DICM}  & 0.5048 & 0.5786 & 0.5807 & 0.5251 & 0.4972 & 0.4991 &  0.6040 & 0.5915 &0.4923& 0.5333 & 0.5827 &\textcolor{blue}{0.6059}  & \textcolor{red}{0.6142}&-\\
    MEF~\cite{MEF}  & 0.5798 & 0.5976 & 0.5949 & 0.5200 & 0.4972 & 0.5177 & 0.6104 & \textcolor{blue}{0.6246} &  0.5946 & 0.4791 & 0.5504 & 0.6175 & \textcolor{red}{0.6282}&-\\
\hline
\end{tabular}}
\end{table*}

\begin{figure}[!t]
    \centering
\setlength{\abovecaptionskip}{0.1cm} %调整caption与图的距离
    \includegraphics[width=1\linewidth]{figs/pdf_user_study.pdf}
    \caption{User studies on DICM and MEF. Our results are preferable to the competing methods. Voting statistics of different methods versus our method.}
    \label{result3}
\end{figure}
% \section{Visualization of Noise-aware Map}

\subsection{Perception Evaluation}
To demonstrate the superior perceptual fidelity of our DPLUT, we utilize the CLIP-IQA~\cite{clip-iqa} for calculating the perception scores of various methods. Specifically, the CLIP-IQA employs paired antonym text prompts (e.g., ``Good photo" and ``Bad photo"). The image and text vectors are generated using the pre-trained CLIP model~\cite{clip}. The CLIP-IQA then calculates the cosine similarity between these vectors, applying a softmax function to derive the perception score, ranging from 0 to 1. A higher score indicates a better quality perception (look) and abstraction perception (feel) of the image. We report the average prediction score of the results from different methods in Table \ref{clip_table}. One can see that, although some methods output impressive results, our DPLUT achieves the best scores and is closer to the ground truth. Consequently, our method yields more perceptual-friendly results compared to alternative approaches.

\subsection{Qualitative Analysis}
In our paper, we have presented comprehensive quantitative results, as detailed in Section \textcolor{red}{5.3}. However, due to limited space, only parts of the visual comparisons are given. Here, we extend our analysis with additional qualitative evaluations against other state-of-the-art (SOTA) methods. Figures \ref{sice_result}, \ref{LOL_result2} and \ref{lsrw2_result} display the enhanced results of SICE~\cite{SICE}, LSRW~\cite{LSRW} and LOL~\cite{RetinexNet}, respectively. One can find that our DPLUT can better balance contrast enhancement, color correction, detail recovery, and naturalness preservation. However, some other comparison methods suffer from color cast, overexposure and underexposure. Some methods (e.g., ZeroDCE~\cite{ZeroDCE} and 3DLUT~\cite{3DLUT}) implement post-processing denoising to mitigate inherent noise in darker regions, but they tend to discard detail in the process. Overall, DPLUT exhibits superior performance in color adjustment, detail preservation and noise suppression, outperforming other compared algorithms. Moreover, we provide more visual comparisons on other well-known benchmarks. Figures \ref{dicm_result} and \ref{dicm_result2} present comparative analyses of the DICM dataset~\cite{DICM}. Figures \ref{mef_result} and \ref{mef_result2} illustrate the qualitative results observed in the MEF dataset~\cite{MEF}. Obviously, across all these comparisons, our method recovers the most authentic tones and provides visual-friendly results, which proves its effectiveness.

\begin{table}[!t]
\centering
\setlength{\abovecaptionskip}{0.1cm} %调整caption与图的距离
\caption{Quantitative evaluation of different methods on the UHD-LL~\cite{UHDFourICLR2023} test set. The best results are highlighted in \textbf{bold} and the second best results are \underline{underlined}. Note that all methods are trained on the LOL~\cite{RetinexNet} training set. The resolution indicates the size of the image that the model processes during inference.}\label{UHD_test}
% \resizebox{8cm}{!}{
\setlength\tabcolsep{2pt}

\begin{tabular}{c|c|cccc}
    \hline	\rowcolor{mygray}	
    Methods & Resolution & PSNR$\uparrow$ & SSIM$\uparrow$ & LPIPS$\downarrow$\\
    \hline	
DRBN~\cite{DRBN} &$3840 \times 2160$ & 16.31 &0.65 & \underline{0.43}\\
3DLUT~\cite{3DLUT} & $3840 \times 2160$ & 14.68 & 0.62 & 0.60 \\
CUE~\cite{3DLUT} & $3840 \times 2160$ & 18.19 & 0.67& 0.54 \\
Retinexformer~\cite{Retinexformer}& $1920 \times 1080$ & 18.49 & 0.73 & 0.48\\
ZeroDCE~\cite{ZeroDCE}& $3840 \times 2160$ & 17.10 & 0.62 & 0.51 \\
ZeroDCE++~\cite{Zerodcepp} &$3840 \times 2160$  & 17.32 & 0.63& 0.49 \\  
RUAS~\cite{RUAS} &$3840 \times 2160$ &  11.76& 0.64 &0.49 \\  
SCI~\cite{SCI} &$3840 \times 2160$ &15.45&  0.57 & 0.51 \\   
PairLIE ~\cite{pairLIE}&$3840 \times 2160$ & 17.53 & 0.66 & 0.49 \\  
NeRCo~\cite{Neco}&$1280 \times 720$ &\underline{19.81}  & \underline{0.74}  & 0.45\\  
CLIP-LIT~\cite{clip-lie}&$3840 \times 2160$ & 15.27 & 0.59 & 0.59 \\ 
\hline
\textbf{DPLUT (Ours)} & $3840 \times 2160$ & \textbf{20.11} & \textbf{0.76}  & \textbf{0.37} \\    
    \hline
\end{tabular}
\end{table}
Furthermore, we evaluate DPLUT with competitive methods that perform well in small-resolution paired datasets on the UHD-LL~\cite{UHDFourICLR2023} test set. UHD-LL test set contains 150 low/normal-light Ultra-High-Definition (UHD) image pairs with 4K ($3840 \times 2160$) resolution. As mentioned in Section \textcolor{red}{5.3} of our paper, some methods (e.g., Retinexformer~\cite{Retinexformer} and CLIP-LIT~\cite{clip-lie}) are unable to handle large-resolution images. Therefore, in alignment with Li et al.~\cite{UHDFourICLR2023}, we downsample the input to the maximum size that the models can handle and then resize the results to the original resolution for performance evaluation. 
The results, as presented in Table \ref{UHD_test}, indicate that DPLUT achieves state-of-the-art (SOTA) quantitative performance, surpassing all methods trained on the LOL~\cite{RetinexNet} dataset. This outcome effectively demonstrates the robust generalization capability of DPLUT in restoring high-resolution low-light images.

\section{Future Works, Limitations and Broader Impacts}
Moving forward, we plan to explore the potential of DPLUT for various tasks while enhancing our overall architecture to make it more efficient and less computationally complex. Our DPLUT shows promising results in handling various light conditions. Nevertheless, a current limitation arises from the necessity of independently optimizing the two lookup tables, LLUT and NLUT, which prevents the full exploitation of their performance. To address this, we intend to implement a joint optimization strategy for both tables, thereby enhancing their collective performance.
DPLUT has exhibited robust performance in low-light conditions, suggesting its applicability across a range of industrial tasks and domains, including surveillance video, autonomous driving, and computational photography. As a result, our research holds significant promise for making a positive impact in both academic and industrial spheres.
